# Supplementary material for: Efficient Subsampled Gauss-Newton and Natural Gradient Methods for Training Neural Networks
Source: arXiv:1906.02353 source file (2019-06-05)
Supplement: Supplementary file 1 [file appendix_not_included.tex]

\centerline{
\bf \LARGE Supplementary Materials (NOT GONNA INCLUDE)
}

\section{Matching loss function}
\label{section_3}

If we choose the nonlinear function of the last layer and the loss function carefully, we can compute $H_i$ in an extremely efficient way. Some typical pairs of nonlinear functions $\phi$ and their matching loss functions $\varepsilon$ that yield efficient computations are:

\begin{enumerate}
	\item Linear $\hat{y} = \phi(h) = h$, and sum-squared loss $\varepsilon(\hat{y}, y) = -||\hat{y} - y||^2$:

    We have that
    \begin{align*}
        & H = -2 I.
    \end{align*}

    \item Logistic $\hat{y} = \phi(h) = \frac{1}{1 + e^{- h}}$, and cross-entropy loss $\varepsilon(\hat{y}, y) = \sum_k y(k) \log \hat{y}(k) + \sum_k (1 - y(k)) \log (1 - \hat{y}(k))$ (Hinton 2006), where $y(k)$ is the $k$-th coordinate of $y$:

    We have that
    \begin{align*}
    	H
        = -\text{diag}(\tilde{y}),
    \end{align*}
    where $\tilde{y}(j) = \hat{y}(j) (1 - \hat{y}(j))$.

    \item Softmax $\hat{y}(j) = \phi(h, j) = \frac{e^{h(j)}}{\sum_k e^{h(k)}}$, and cross-entropy loss $\varepsilon(\hat{y}, y) = - \sum_k y(k) \log \hat{y}(k)$:

	When $\sum_k y(k) = 1$, we have that
    \begin{align*}
    	H
        & = - \left( \text{diag}(\hat{y}) - \hat{y} \hat{y}^T \right).
    \end{align*}

\end{enumerate}

\subsection{Detailed computation of the Hessian of matching loss function}

Throughout this section, we consider a single data point, and we omit the subscript $i$. If we view $f $ as a function of $\hat{y}$, then
$$f(\hat{y}) = \varepsilon(\hat{y}, y).$$

\begin{enumerate}
	\item Linear $\hat{y} = \phi(h) = h$, sum-squared loss $\varepsilon(\hat{y}, y) = -||\hat{y} - y||^2$:

    Then,
    \begin{align*}
    	& \varepsilon = -||h - y||^2
    	\\ \Rightarrow & \frac{\partial \varepsilon}{\partial h} = -2 (h - y)
        \\ \Rightarrow & \frac{\partial^2 \varepsilon}{\partial h^2} = -2 I.
    \end{align*}

    \item Logistic $\hat{y} = \phi(h) = \frac{1}{1 + e^{- h}}$,
    %cross-entropy loss $\varepsilon(\hat{y}, y) = - \sum_k y(k) \log \hat{y}(k)$,
    cross-entropy loss $\varepsilon(\hat{y}, y) = \sum_k y(k) \log \hat{y}(k) + \sum_k (1 - y(k)) \log (1 - \hat{y}(k))$ (Hinton 2006),
    where $y(k)$ is the $k$-th coordinate of $y$:

    Then,
    \begin{align*}
    	\varepsilon
        %& = - \sum_k y(k) \log \hat{y}(k) - \sum_k (1 - y(k)) \log (1 - \hat{y}(k))
        %& = - \sum_k y(k) \log \frac{1}{1 + e^{- h(k)}} - \sum_k (1 - y(k)) \log \left(1 - \frac{1}{1 + e^{- h(k)}} \right)
        %& = \sum_k y(k) \log (1 + e^{- h(k)}) - \sum_k (1 - y(k)) \log \left(1 - \frac{1}{1 + e^{- h(k)}} \right)
        %& = -\sum_k y(k) \log (1 + e^{- h(k)}) + \sum_k (1 - y(k)) \log \left( \frac{e^{- h(k)}}{1 + e^{- h(k)}} \right)
        %\\ & = \sum_k y(k) \log (1 + e^{- h(k)})
        %\\ & - \sum_k (1 - y(k)) \log ( e^{- h(k)} ) + \sum_k (1 - y(k)) \log ( 1 + e^{- h(k)} )
        & = -\sum_k \log (1 + e^{- h(k)}) - \sum_k (1 - y(k)) h(k).
    \end{align*}
    Hence,
    \begin{align*}
    	\frac{\partial \varepsilon}{\partial h(j)}
        & = -\frac{1}{1 + e^{- h(j)}} e^{- h(j)} (-1) - (1 - y(j))
        \\ & = -\frac{1}{1 + e^{- h(j)}} + y(j).
        \\ & \left( = -\hat{y}(j) + y(j) \right)
    \end{align*}
    Furthermore,
    \begin{align*}
    	\frac{\partial^2 \varepsilon}{\partial h(j)^2}
        & = \frac{1}{(1 + e^{- h(j)})^2} e^{- h(j)} (-1)
        %\\ & = \frac{1}{(1 + e^{- h(j)})^2} e^{- h(j)}
        \\ & = -\hat{y}(j) \left( 1 - \hat{y}(j) \right).
    \end{align*}

    If we denote $\tilde{y}(j) = \hat{y}(j) (1 - \hat{y}(j))$,
    \begin{align*}
    	\frac{\partial^2 \varepsilon}{\partial h^2}
        = -\text{diag}(\tilde{y}).
    \end{align*}

    \item
    Softmax $\hat{y}(j) = \phi(h, j) = \frac{e^{h(j)}}{\sum_k e^{h(k)}}$, cross-entropy loss $\varepsilon(\hat{y}, y) = \sum_k y(k) \log \hat{y}(k)$:

    Then,
    \begin{align*}
    	\varepsilon
        %& = - \sum_j y(j) \log \hat{y}(j)
        & = \sum_r y(r) \log \left( \frac{e^{h(r)}}{\sum_k e^{h(k)}} \right)
        %\\ & = - \sum_j y(j) \left( \log \left( e^{h(j)} \right) - \log \left( \sum_k e^{h(k)} \right) \right)
        \\ & = \sum_r y(r) \left( h(r) - \log \left( \sum_k e^{h(k)} \right) \right)
        %\\ & = - \sum_j \left( y(j) h(j) - y(j) \log \left( \sum_k e^{h(k)} \right) \right)
        %\\ & = - \left( \sum_j y(j) h(j) - \sum_j y(j) \log \left( \sum_k e^{h(k)} \right) \right)
        %\\ & = - \sum_j y(j) h(j) + \sum_j y(j) \log \left( \sum_k e^{h(k)} \right)
        \\ & = \sum_r y(r) h(r) + \log \left( \sum_k e^{h(k)} \right) \cdot \sum_r y(r)
        \\ & = \sum_k y(k) h(k) + \log \left( \sum_k e^{h(k)} \right) \cdot \sum_k y(k).
    \end{align*}
    Hence,
    \begin{align*}
    	\frac{\partial \varepsilon}{\partial h(j)}
        %& = \frac{\partial \left( - \sum_j y(j) h(j) + \log \left( \sum_k e^{h(k)} \right) \cdot \sum_j y(j) \right)}{\partial h(j)}
        & = - y(j) + \sum_k y(k) \cdot \frac{1}{\sum_k e^{h(k)}} \cdot e^{h(j)}.
        \\ & \left( = - y(j) + \sum_k y(k) \cdot \hat{y}(j) \right)
    \end{align*}

    For $l \neq j$,
    \begin{align*}
    	\frac{\partial^2 \varepsilon}{\partial h(l) \partial h(j)}
        & = \frac{\partial \left( \frac{\partial \varepsilon}{\partial h(j)} \right) }{\partial h(l)}
        %\\ & = \frac{\partial \left( - y(j) + \sum_j y(j) \cdot \frac{1}{\sum_k e^{h(k)}} \cdot e^{h(j)} \right) }{\partial h(l)}
        %\\ & = \frac{\partial \left( \sum_j y(j) \cdot \frac{1}{\sum_k e^{h(k)}} \cdot e^{h(j)} \right) }{\partial h(l)}
        %\\ & = \sum_j y(j) \cdot \frac{\partial \left( \frac{1}{\sum_k e^{h(k)}} \cdot e^{h(j)} \right) }{\partial h(l)}
        \\ & = \left( \sum_k y(k) \right) \cdot e^{h(j)} \cdot \frac{\partial \left( \frac{1}{\sum_k e^{h(k)}} \right) }{\partial h(l)}
        \\ & = \left( \sum_k y(k) \right) \cdot e^{h(j)} \cdot (-1) \frac{1}{(\sum_k e^{h(k)})^2} e^{h(l)}
        %\\ & = -\sum_j y(j) \cdot e^{h(j)} \cdot \frac{1}{(\sum_k e^{h(k)})^2} e^{h(l)}
        \\ & = -\left( \sum_k y(k) \right) \cdot \hat{y}(j) \cdot \hat{y}(l).
    \end{align*}
    Besides,
    \begin{align*}
    	& \frac{\partial^2 \varepsilon}{\partial h(j)^2}
        = \frac{\partial \left( \frac{\partial \varepsilon}{\partial h(j)} \right) }{\partial h(j)}
        %\\ & = \frac{\partial \left( - y(j) + \sum_j y(j) \cdot \frac{1}{\sum_k e^{h(k)}} \cdot e^{h(j)} \right) }{\partial h(j)}
        %\\ & = \frac{\partial \left( \sum_j y(j) \cdot \frac{1}{\sum_k e^{h(k)}} \cdot e^{h(j)} \right) }{\partial h(j)}
        \\ = & \left( \sum_k y(k) \right)
        \\ & \cdot \left( \frac{\partial \left( \frac{1}{\sum_k e^{h(k)}} \right) }{\partial h(j)} \cdot e^{h(j)}
        + \frac{1}{\sum_k e^{h(k)}} \cdot \frac{\partial \left( e^{h(j)} \right) }{\partial h(j)} \right)
        \\ & = \left( \sum_k y(k) \right)
        \\ & \cdot \left( (-1) \frac{1}{(\sum_k e^{h(k)})^2} e^{h(j)} \cdot e^{h(j)} + \frac{1}{\sum_k e^{h(k)}} \cdot e^{h(j)} \right)
        \\ & = \left( \sum_k y(k) \right) \cdot \left( - \hat{y}(j)^2 + \hat{y}(j) \right).
    \end{align*}
    Hence,
    \begin{align*}
    	\frac{\partial^2 \varepsilon}{\partial h^2}
        & = \left( \sum_k y(k) \right) \cdot \left( \text{diag}(\hat{y}) - \hat{y} \hat{y}^T \right).
    \end{align*}
    Usually, $y$ denotes a probability distribution. Hence, $\sum_k y(k) = 1$. We have that
    \begin{align*}
    	\frac{\partial^2 \varepsilon}{\partial h^2}
        & = -(\text{diag}(\hat{y}) - \hat{y} \hat{y}^T),
    \end{align*}
    which is not invertible. Adding a small perturbation makes it invertible, which gives us
    \begin{align*}
        & \left( \text{diag}(\hat{y}) - \hat{y} \hat{y}^T + c I \right)^{-1}
        \\ = & \left( \text{diag}(\hat{y} + c) - \hat{y} \hat{y}^T \right)^{-1}
        \\ = & \text{diag}(\hat{y} + c)^{-1}
        \\ & - \text{diag}(\hat{y} + c)^{-1} \hat{y} \left( -1 + \hat{y}^T \text{diag}(\hat{y} + c)^{-1} \hat{y} \right)^{-1} \hat{y}^T \text{diag}(\hat{y} + c)^{-1}
    \end{align*}

\iffalse
During one iteration, the running time is:
\begin{enumerate}
\item $\alpha_k = \frac{r_k^T r_k}{p_k^T B p_k}$: $4 k n + 2 k^2 + 6 n$.

\item $x_{k+1} = x_k + \alpha_k p_k$: $2 n$.

\item $r_{k+1} = r_k - \alpha_k B p_k$: $2 n$ ($B p_k$ can be stored after step 1).
\item $\beta_k = \frac{r_{k+1}^T r_{k+1}}{r_{k}^T r_{k}}$: $4 n$.

\item $p_{k+1} = r_{k+1} + \beta_k p_k$: $2 n$.
\end{enumerate}
In sum, the running time is $4 k n + 16 n + 2 k^2$.
\fi

\end{enumerate}
